# Supplementary material for: Stochastic Package Queries in Probabilistic Databases
Source: arXiv:2103.06784 source file (2021-03-11)
Supplement: Supplementary file 1 [file direct.tex]

An \emph{exact} translation
is a procedure that transforms a \spaql query into an equivalent integer program
that is readily solvable by an existing solver.
Because solvers typically employ heuristics and approximations,
the actual result may, in practice, be not exact.
Our discussion abstracts from solver-specific features
and only concentrates on the exactness of the final problem formulation.

The SP literature has long studied exact formulations~\cite{birge2011introduction}.
Typically, they are only possible under certain, very restrictive conditions,
such as the ability to perform multi-variate integration.
Even seemingly simple cases, such as Gaussian variables,
hide nontrivial system challenges.

Covering all results in this area is outside the scope of this paper.
We show an exact formulation only applicable under these conditions:
(1)~The objective function is either deterministic or an expectation (not probabilistic).
(2)~The expected value of all random variables involved in the expectation objective
and all expectation constraints is known exactly
or it can be analytically derived.
For example, all random tuple values
follow a Poisson distribution with known (and possibly different) means.
(3)~All random variables involved in a probabilistic constraint follow Gaussian distributions,
with known expectation and variance, and if the random variables have correlation,
their covariance is also known exactly.
Further, in every probabilistic constraint, $p$ is greater than or equal to $0.5$
(for the constraint to be convex, as discussed below).

\subsection{Exact Formulation} \label{subsec:exact-normal}

We assume that the expected value and standard deviation of $t.\attr{A}$, if known,
are stored in the input table as deterministic attributes, $t.\mu_{\attr{A}}$ and $t.\sigma_{\attr{A}}$, respectively.
If the random variables have correlation,
we assume that all non-zero covariances are stored in a table $\rel{R\_Covariance}(\attr{A})$,
where tuple $\sigma_{i_1 i_2}.\attr{A}$ stores the covariance between $\tuple_{i_1}.\attr{A}$ and $\tuple_{i_2}.\attr{A}$.
The exact translation does not use Monte Carlo simulations and, thus, it never calls any of the VG functions.

\para{Expectations}
Because of linearity of expectations,
$\expe{\sum_{i=1}^{N} t_i.\attr{A}\; x_i} = \sum_{i=1}^{N} \expe{t_i.\attr{A}} x_i = \sum_{i=1}^{N} t_i.{\mu_{\attr{A}}}\; x_i$.
Therefore, an expectation function is simply replaced with its analogous deterministic
predicate over the expected values.

\para{Probabilistic constraints with Gaussian tuples}
Consider a probabilistic constraint on a Gaussian attribute $\attr{A}$ of the form
$\prob{\sum_{i=1}^{N} t_i.\attr{A}\; x_i \ge v} \ge p$.
Assume for now that all tuples are independent (we relax this assumption later).
Known SP results~\cite{ahmed2008solving,kall1994stochastic,kataoka1963stochastic,shapiro2009lectures}
show that, if $p \in [0.5,1]$, this constraint is convex
(specifically, ``second-order cone'') and equivalent to the following deterministic constraint:
\begin{equation} \label{eq:gaussian-large}
\textstyle\sum_{i=1}^{N} \tuple_i.\mu_{\attr{A}} * x_i
\ge v + z_p \sqrt{\textstyle\sum_{i=1}^{N} \tuple_i.\sigma_{\attr{A}}^2 * x_i^2}
\end{equation}
where $z_p = \Phi^{-1}(p) \in \reals$ is the $p$-quantile (inverse CDF of $p$) of the standard Gaussian distribution.
Second-order cone constraints can be solved by most solvers (e.g., IBM \cplex~\cite{cplex}).
However, they typically accept these constraints in a different, simpler form.
A known technique for feeding these constraints to solvers (e.g,~\cite{franco2015robust})
involves rewriting~\Cref{eq:gaussian-large}
into an equivalent set of constraints that solvers accept.
We first introduce a new continuous variable $c$ into the integer program, and
add a new linear constraint on the expectation:
\begin{equation} \label{eq:gaussian-mu}
\textstyle\sum_{i=1}^{N} \tuple_i.\mu_{\attr{A}} * x_i \ge v + z_p c
\end{equation}
Then, we add the following quadratic constraint on the standard deviation:
\begin{equation} \label{eq:independent-gaussian-sigma}
\textstyle\sum_{i=1}^{N} \tuple_i.\sigma_{\attr{A}}^2 * x_i^2 \le c^2
\end{equation}
Constraint~\ref{eq:independent-gaussian-sigma} is also second-order cone, but in a form that most solvers accept.

\begin{proposition}
Constraints~(\ref{eq:gaussian-mu}) and~(\ref{eq:independent-gaussian-sigma})
are equivalent to constraint~(\ref{eq:gaussian-large}).
\end{proposition}
\begin{proof}
    (\ref{eq:gaussian-large})$\Rightarrow$(\ref{eq:gaussian-mu})$\land$(\ref{eq:independent-gaussian-sigma}):
    Setting $c^2 \coloneqq \textstyle\sum_{i=1}^{N} \tuple_i.\sigma_{\attr{A}}^2 * x_i^2$
    immediately implies~(\ref{eq:gaussian-mu}), and also that
    $c^2 \ge \textstyle\sum_{i=1}^{N} \tuple_i.\sigma_{\attr{A}}^2 * x_i^2$~(\ref{eq:independent-gaussian-sigma}).
    (\ref{eq:gaussian-mu})$\land$(\ref{eq:independent-gaussian-sigma})$\Rightarrow$(\ref{eq:gaussian-large}):
    Immediate consequence.
\end{proof}

With correlation among the variates,~\Cref{eq:independent-gaussian-sigma} becomes:
\begin{equation} \label{eq:correlated-gaussian-sigma}
\textstyle\sum_{i_1=1}^{N}\sum_{i_2=1}^{N} \sigma_{i_1 i_2}.{\attr{A}} * x_{i_1} * x_{i_2} \le c^2,
\end{equation}
which is only practical if $\rel{R\_Covariance}$ is sparse.
Otherwise, the left-hand side of~\Cref{eq:correlated-gaussian-sigma} may get as large as $N^2$,
making it too large to fit in main memory.

\para{Size complexity}
We measure size complexity in terms of the number of coefficients added to the problem
as a function of the number of tuples, $N$.
The exact translation adds $N$ coefficients for each expectation function,
$2N+2$ coefficients for each probabilistic constraint without correlation, and
$O(N^2)$ coefficients for each probabilistic constraint with correlation.

\subsection{Exact Query Evaluation} \label{subsec:direct-query-eval}
Query evaluation when an exact formulation is possible is very simple.
Given a \spaql query $\query$:
\begin{enumerate}[wide,labelwidth=!,labelindent=0pt,itemsep=2pt,topsep=5pt]
    \item
    Translate $\query$ into the equivalent deterministic integer program
    as dictated by the aforementioned translation rules.
    \item
    Solve the resulting integer program using an off-the-shelf integer programming solver
    capable of handling the resulting linear (or quadratic) constraints (e.g., IBM \cplex),
    obtaining a solution for each of the integer variables $x_i$.
    \item
    Construct the result package by including each tuple $t_i$ as many times as the value of $x_i$
    (if $x_i = 0$, $t_i$ is not included in the package at all).
\end{enumerate}
