# Supplementary material for: Stochastic Package Queries in Probabilistic Databases
Source: arXiv:2103.06784 source file (2021-03-11)
Supplement: Supplementary file 2 [file proofs.tex]

\subsubsection*{Feasibility Guarantees}

\begin{proof}[Proof of \Cref{thm:feasibility}]
    Let $\rho(k;n,p)$
    be the probability of having less than $k$ successes in $n$ i.i.d. trials,
    each with probability $p$ of success:
    \begin{equation*}
    \rho(k;n,p) \coloneqq \textstyle\sum_{i=0}^{\floor{k}}\binom{n}{i}p^i(1-p)^{n-i}.
    \end{equation*}
    We show the analysis for a single probabilistic constraint with right-hand side $p$.
    The same result applies to each individual constraint.
    Suppose there exists a \vfeasible solution $x$, i.e., $1/\hat{M}\sum_{j=1}^{\hat{M}}\hat{Y}_j \ge p$,
    where $\hat{Y}_j$ is the event ``$x$ satisfies the $j^\text{th}$ validation scenario''.
    $\CSAsolve(\query, M, Z)$ fails in finding a \vfeasible solution iff
    every SSA formulation is infeasible or every solution produced by an SSA formulation
    is \vinfeasible.
    There are exactly $M/Z$ possible SSA formulations in the search space of $\CSAsolve(\query, M, Z)$,
    one for each possible value that $\alpha$ can take
    (the ordering of the scenarios does not matter for the analysis).
    Let the $n^\text{th}$ SSA formulation be $\CSA_n$,
    where $\CSA_n$ uses $\alpha(n) = nZ/M$, for $n = 1, \dots, M/Z$.

    We first establish the probability that every $\CSA_n$ is infeasible.
    Because $x$ is \vfeasible, $\probs{\hat{Y}_j = 1} \ge p$.
    Because $\hat{M} \gg M$, $\probs{Y_j = 1} \ge p$,
    where $Y_j$ is the event ``$x$ satisfies the $j^\text{th}$ optimization scenario'',
    and thus $\probs{Y_j \le 0} < 1- p$.
    Since $\alpha(n) = nZ/M$, each individual summary is the min (or max) of $n$ real optimization scenarios.
    Suppose the summary is the min of $n$ scenarios.
    Then, because scenarios are i.i.d.,
    $\probs{\min_{j=1,\dots,n}\{Y_j\} \le 0} = 1 - (1 - \probs{Y_j \le 0})^n < 1 - p^{n}$.
    Similarly, for a max summary we get
    $\probs{\max_{j=1,\dots,n}\{Y_j\} \le 0} = \probs{Y_j \le 0}^n < (1-p)^n \le 1 - p^{n}$.
    Therefore, each summary is satisfied by $x$ with probability at least $p^{n}$.
    The probability of $\CSA_n$ being infeasible is the probability of having
    less than $p\%$ satisfiable summaries,
    which is equal to having less than $pZ$ successes in $Z$ trials, each
    having probability at least $p^{n}$,
    i.e. $\probs{SSA_n \text{ is infeasible}} \le \rho(pZ; Z, p^{n})$.
    Because $\forall n: pZ \le p^{n}Z$, using Hoeffding's inequality~\cite{Hoeffding1963} we have that
    $\rho(pZ; Z, p^{n}) \le \exp(-2 Z (p^{n} - p)^2)$.
    Therefore, $\probs{\text{every } SSA_n \text{ is infeasible}} \le \prod_{n=1}^{M/Z} \rho(pZ; Z, p^{n})
    \le \prod_{n=1}^{M/Z} \exp(-2 Z (p^{n} - p)^2)$,
    which decreases exponentially with increasing $M$ or decreasing $Z$.

    We now establish the probability that every feasible $\CSA_n$ returns a solution $x_n$ that is \vinfeasible.
    Let $S_z$ be the event ``$x_n$ satisfies the $z^\text{th}$ summary''.\
    By definition of $\CSA_n$, $\prob{S_z=1} \ge p$.
    By the summary construction, if a summary is satisfied, at least $n$ real optimization scenarios are also satisfied.
    Therefore, $\probs{Y_j=1 \mid S_z=1} \ge n/M$.
    Also, $\prob{S_z=1 \mid Y_j=1} = 1/Z$
    because satisfying a real scenario does not imply satisfying a summary (only the opposite is true).
    Applying Bayes' rule,
    $\prob{Y_j=1} = \probs{Y_j=1 \mid S_z=1}\probs{S_z=1}/\prob{S_z=1 \mid Y_j=1} \ge pnZ/M = p\alpha(n)$.
    Because scenarios are i.i.d., the same probability is maintained in the larger, out-of-sample,
    validation set, thus $\probs{\hat{Y}_j=1} \ge p\alpha(n)$.
    It follows that the probability of $x_n$ being \vinfeasible is equal to
    having less than $p\hat{M}$ successes in $\hat{M}$ trials,
    each having a probability of $p\alpha(n)$.
    Therefore, $\probs{x_n \text{ is \vinfeasible}} \le \rho(p\hat{M}; \hat{M}, p\alpha(n))$.
    Because $\forall n : p\hat{M} \le p \alpha(n) \hat{M}$,
    applying Hoeffding's inequality we obtain
    $\rho(p\hat{M}; \hat{M}, p\alpha(n)) \le \exp(-2 \hat{M} (p\alpha(n) - p)^2)$.
    Therefore, $\probs{\text{every } x_n \text{ is \vinfeasible}}
    \le \prod_{n=1}^{M/Z} \rho(p\hat{M}; \hat{M}, p\alpha(n))
    \le \prod_{n=1}^{M/Z} \exp(-2 \hat{M} (p\alpha(n) - p)^2)$,
    which decreases exponentially with increasing $M$ or decreasing $Z$.

    Thus, increasing $M$ exponentially reduces the chance that all SSA problems are infeasible
    and that all the feasible ones only produce \vinfeasible solutions,
    exponentially increasing the chance of \CSAsolve to find at least one \vfeasible solution.
\end{proof}

\subsubsection*{Convergence Guarantees}

\begin{proof}[Proof of \Cref{th:convergence}]
    First, we prove that for every probabilistic constraint $C_k$,
    the conservativeness will eventually converge to some $\alpha_k^{(\hat{n})}$, at some iteration $\hat{n}$.
    At every iteration $n$, \CSAsolve fits an arctangent to the history of $p$-surplus values,
    $H_k = \{(\alpha_k^{(n')}, r_k^{(n')}) \mid n' < n\}$.
    By definition of $p$-surplus, all $p$-surplus values have the same underlying distribution,
    conditioned on the conservativeness level $\alpha_k^{(n')}$.
    The history is therefore a sample from this distribution.
    \CSAsolve uses least squares regression to fit the arctangent,
    finds the root $\alpha_k^*$ of the fit function,
    and discretizes it as $\alpha_k^{(n)} \coloneqq \ceil{\alpha_k^*}$.
    The resulting curve minimizes the least squared error,
    and thus approximates the expectation of the $p$-surplus conditioned on the conservativeness.
    By the weak law of large numbers, the larger the history, the better the curve approximates
    the true expectation curve.
    Eventually, with a large enough history, starting at some iteration $\hat{n}$,
    adding more data points to the history will not change the fit curve
    enough for its discretized root $\ceil{\alpha_k^*}$ to change.

    If \CSAsolve does not reorder the scenarios at each iteration,
    the algorithm will stop at this point.
    Otherwise, because summaries are constructed to ensure monotonicity of the objective value
    with changes to the conservativeness,
    after iteration $\hat{n}$, the solution can only improve in objective value or remain the same.
    Because there is finite number of possible reordering of the optimization scenarios,
    the objective value cannot indefinitely improve,
    and the solution will converge to a local optimum,
    terminating the algorithm.
\end{proof}

\begin{proof}[Proof of \Cref{th:convergence-sss}]
    First, because of \Cref{th:convergence}, every iteration of \sss terminates with a solution.
    With $M'$ scenarios and $M'$ summaries, there is only one possible SSA problem: $\CSA_{M',M'}$.
    This problem is identical to $\SAA_{M'}$, used by \naive with $M'$ scenarios.
    \Cref{thm:feasibility} establishes that when $Z$ decreases,
    the probability of the corresponding SSA problem produces a \vfeasible solution increases.
    Because at $Z=M'$ the solution is already \vfeasible (with probability 1),
    for all $Z' \le M'$, the obtained SSA solutions will also be \vfeasible (with probability 1).
    Therefore, regardless of $Z$, \sss will never increase $M$ above $M'$, for a maximum of $\ceil{M'/m}$
    increments.
    Similarly, $Z$ will only increase by at most $\ceil{M'/z}$ increments.
    Therefore, \sss is guaranteed to terminate with the same solution obtained by \naive
    in at most $\ceil{M'/m} + \ceil{M'/z} \le 2M'$ iterations,
    a factor of at most 2 compared to \naive.
\end{proof}

\subsubsection*{Approximation Guarantees}

\para{Definitions}
Let $\hat{s}_{ij}$ be the $j^\text{th}$ validation scenario for tuple $t_i$,
and let $\underline{s} \coloneqq \min_{i,j}\{\hat{s}_{ij}.\attr{A}\}$ be the smallest such value.
Let $x$ be any solution.
We denote with $\hat{S}_{x} \coloneqq \{j : \sum_{i=1}^{N} \hat{s}_{ij}.\attr{A}\; x_i \odot v, 1 \le j \le \hat{M}\}$
the set of validation scenarios satisfied by $x$,
and with $\hat{U}_x \coloneqq \{j : j \notin \hat{S}_x\}$ the unsatisfied ones.
Let $\gamma(x) \coloneqq \sum_{i=1}^{N}\sum_{j \in \hat{S}_{x}} (1/\hat{M})\; \hat{s}_{ij}.\attr{A}\; {x}_i$.
The aggregate function $\gamma(x)$ is efficiently computed as part of the validation procedure.
We first prove the following lemma.

\begin{lemma} \label{lm:unsupportive}
    For any unsupportive probabilistic constraint,
    \begin{align} \label{eq:mu-bounds}
    \omega^{(\hat{n})} < \begin{cases}
        \gamma(x^{(\hat{n})}) + (1-p)v  & \text{if}~v \ge 0 \\
        \gamma(x^{(\hat{n})})           & \text{if}~v < 0
    \end{cases}
    \end{align}
\end{lemma}

\begin{lemma} \label{lm:unsupportive2}
    For any unsupportive probabilistic constraint,
    if no scenario value is negative (i.e., $\underline{s} \ge 0$),
    \begin{align} \label{eq:mu-bounds-hat}
    \hat{\omega} \ge \begin{cases}
        pv  & \text{if}~v \ge 0 \\
        v   & \text{if}~v < 0,
    \end{cases}
    \end{align}
    otherwise (i.e., $\underline{s} < 0$),
    \begin{align} \label{eq:mu-bounds-hat}
    \hat{\omega} \ge \begin{cases}
        pv + (1-p)\underline{s}  & \text{if}~v \ge 0 \\
        v + (1-p)\underline{s}   & \text{if}~v < 0
    \end{cases}
    \end{align}
\end{lemma}

\begin{proof}[Proof of \Cref{lm:unsupportive}]
    We show the full proof for the case $v \ge 0$.
    \begin{align*}
        \omega^{(\hat{n})}
        &= 1/\hat{M} \left(
        \textstyle\sum_{j=1}^{\hat{M}} \textstyle\sum_{i=1}^{N} \hat{s}_{ij}.\attr{A}\; x_i
        \right) \\
        &= 1/\hat{M} \left(
        \textstyle\sum_{j \in \hat{S}_x} \textstyle\sum_{i=1}^{N} \hat{s}_{ij}.\attr{A}\; x_i +
        \textstyle\sum_{j \notin \hat{S}_x} \textstyle\sum_{i=1}^{N} \hat{s}_{ij}.\attr{A}\; x_i
        \right) \\
        &< 1/\hat{M} \left(
        \textstyle\sum_{j \in \hat{S}_x} \textstyle\sum_{i=1}^{N} \hat{s}_{ij}.\attr{A}\; x_i +
        \textstyle\sum_{j \notin \hat{S}_x} v
        \right) \\
        &= 1/\hat{M} \left(
        \textstyle\sum_{j \in \hat{S}_x} \textstyle\sum_{i=1}^{N} \hat{s}_{ij}.\attr{A}\; x_i +
        |\hat{U}_x| v
        \right) \\
        &\le 1/\hat{M} \left(
        \textstyle\sum_{j \in \hat{S}_x} \textstyle\sum_{i=1}^{N} \hat{s}_{ij}.\attr{A}\; x_i +
        (1-p)\hat{M} v
        \right) \\
        &= \gamma(x^{(\hat{n})}) + (1-p) v
    \end{align*}
    where we used the fact that, since $\omega^{(\hat{n})}$ is \vfeasible,
    it cannot break more than $(1-p)\hat{M}$ validation scenarios, i.e., $|\hat{U}_x| \le (1-p)\hat{M}$.
    To prove the case where $v < 0$, we use that $|\hat{U}_x| \ge 0$.
\end{proof}

\begin{proof}[Proof of \Cref{lm:unsupportive2}]
    We show the full proof for the case $v \ge 0$, $\underline{s} \ge 0$.
\begin{align*}
    \hat\omega
    &= 1/\hat{M} \left(
    \textstyle\sum_{j=1}^{\hat{M}} \textstyle\sum_{i=1}^{N} \hat{s}_{ij}.\attr{A}\; \hat{x}_i
    \right) \\
    &= 1/\hat{M} \left(
    \textstyle\sum_{j \in \hat{S}_{\hat{x}}} \textstyle\sum_{i=1}^{N} \hat{s}_{ij}.\attr{A}\; \hat{x}_i +
    \textstyle\sum_{j \notin \hat{S}_{\hat{x}}} \textstyle\sum_{i=1}^{N} \hat{s}_{ij}.\attr{A}\; \hat{x}_i
    \right) \\
    &\ge 1/\hat{M} \left(
    \textstyle\sum_{j \in \hat{S}_{\hat{x}}} v
    \right) \\
    &= 1/\hat{M} \left(
    |\hat{S}_{\hat{x}}| v
    \right) \\
    &\ge 1/\hat{M} \left(
    p \hat{M} v
    \right) \\
    &= pv
\end{align*}
    where we used that, for any feasible solution $x'$,
    $|\hat{S}_{x'}| \ge p\hat{M}$ and
    $0 \le |\hat{U}_{x'}| \le (1-p)\hat{M}$.
\end{proof}

\begin{proof}[Proof of \Cref{th:unsupp-approx-mc}]
    \Cref{eq:gamma-bound} can be rewritten as:
    \begin{equation*}
    \gamma(x, \hat{S}_x) + (1-p)v \le ({1+\epsilon})pv
    \end{equation*}
    Plugging \Cref{eq:mu-bound} and \Cref{eq:muhat-bound} immediately proves the theorem.
\end{proof}
